# Supplementary material for: Choose What You Need: Disentangled Representation Learning for Scene Text Recognition, Removal and Editing
Source: arXiv:2405.04377 source file (2024-05-07)
Supplement: Supplementary file 1 [file X_suppl.tex]

\clearpage
\setcounter{page}{1}
\maketitlesupplementary

\begin{figure*}[!h]
  \centering
   \includegraphics[width=1.0\linewidth]{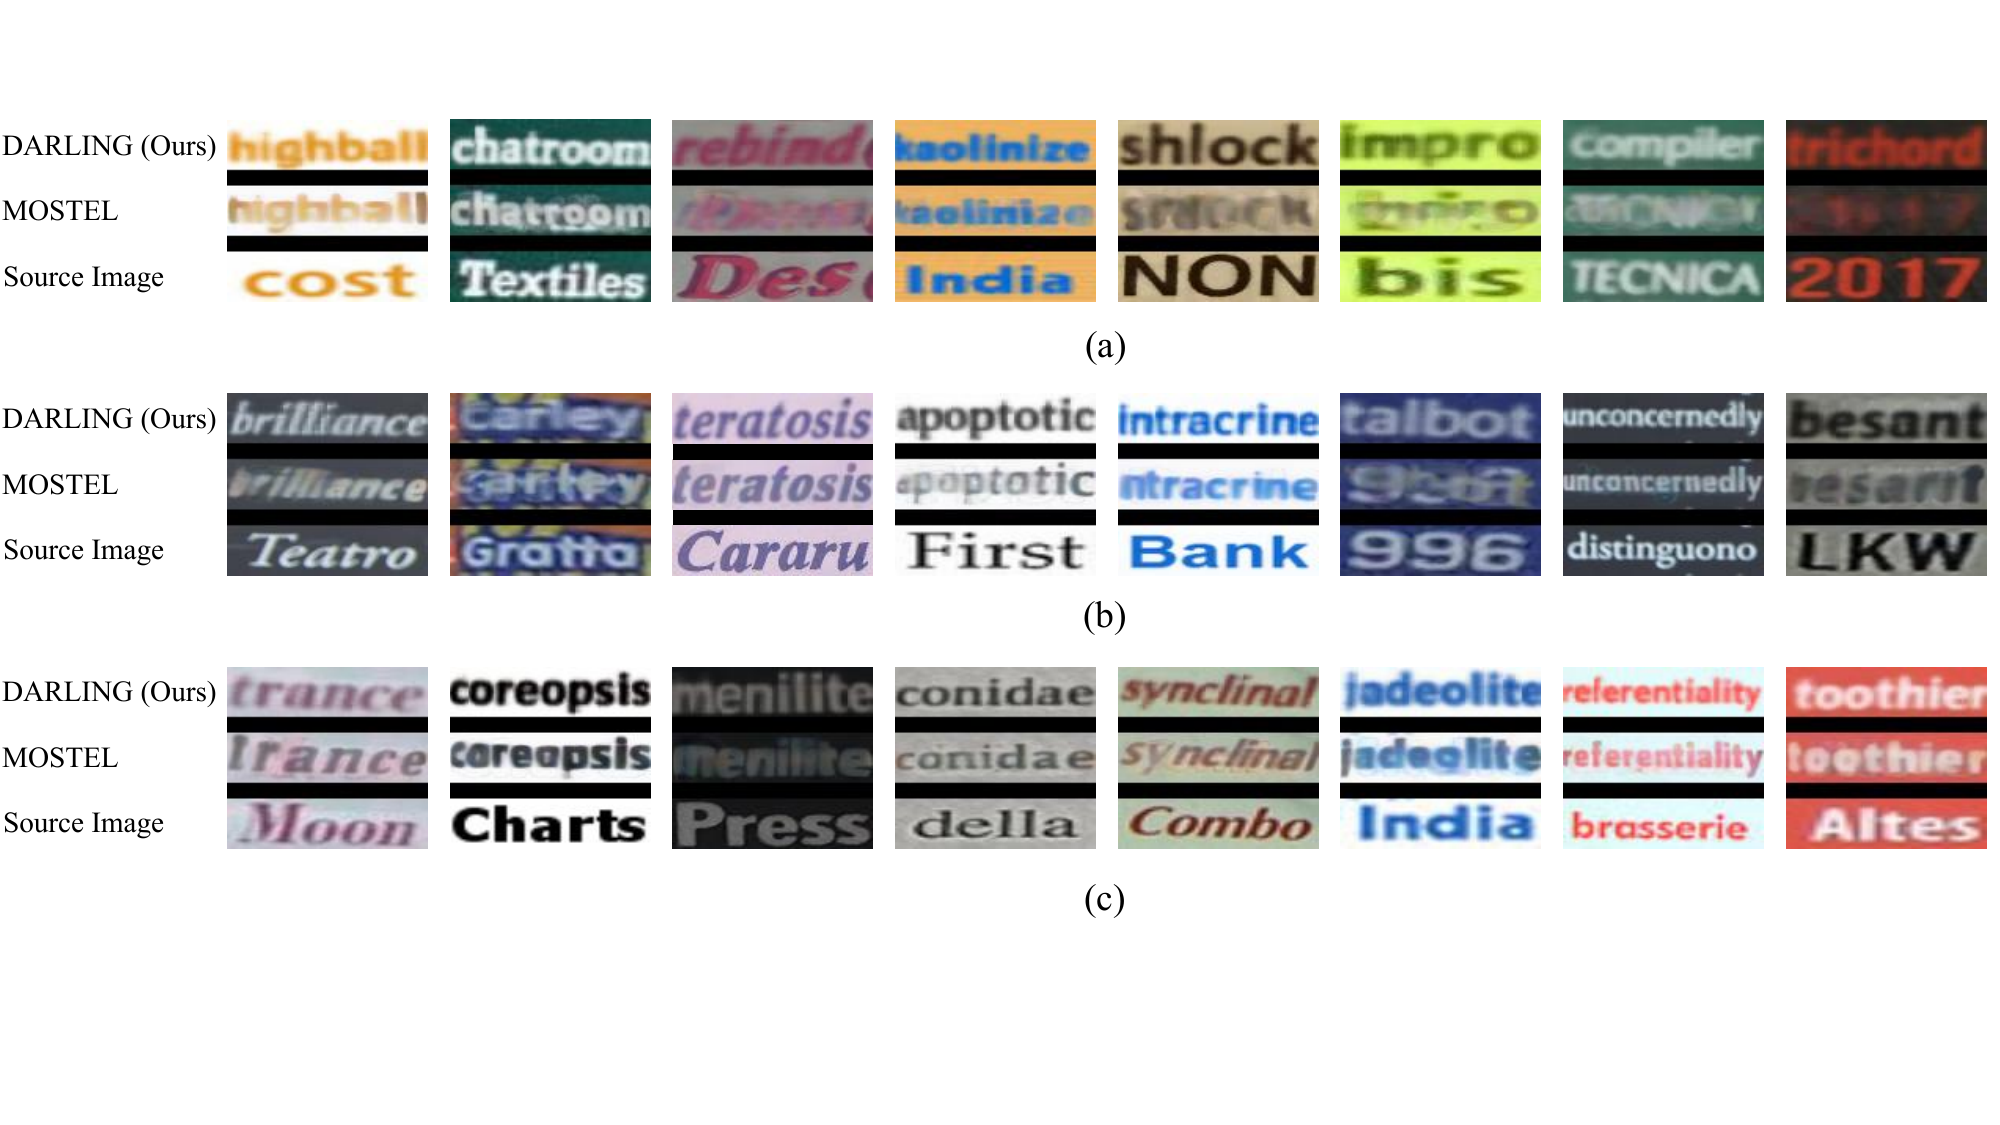}
   \caption{Comparisons of generated instances in scene text editing. (a) Comparison of the generation quality. (b) Comparison of the style transfer ability. (c) Comparison of the authenticity of generated images.}
   \label{fig:ste_more}
\end{figure*}

\section{More Implementation Details}
\subsection{Details about Text Prompt}
Within our Multi-task Decoder (MTD), we employ a text prompt $\mathbf{C}_T$ to direct the generation branch in producing edited text images. The text prompt specifies the desired text to be rendered onto the image. We use a learnable embedding layer to transform the texts into a text prompt. The category number of the embedding layer is 96 which represents 96 characters.

\subsection{Details about ClassAcc}
The legibility and clarity of generated images do not necessarily guarantee high authenticity. Consequently, we introduce a metric termed ClassAcc to assess the authenticity of generated images. This metric employs a simple convolutional network to evaluate the authenticity of both generated and original images. The training dataset comprises both original and generated images, and the network undergoes training for 50 epochs. The classification accuracy serves as an indicator of the authenticity of generated images. The code for the classification network is provided below.

\begin{lstlisting}
class ClassAcc(nn.Module):
    def __init__(self):
        super().__init__()
        self.conv1 = nn.Conv2d(3,32, kernel_size=3, stride=2, padding=1)
        self.relu = nn.ReLU()
        self.conv2 = nn.Conv2d(32,32, kernel_size=3, stride=2, padding=1)
        self.pred = nn.Linear(32,2)

    def forward(self, x):
        x = self.relu(self.conv1(x))
        x = self.relu(self.conv2(x))
        x = torch.mean(x, dim=(2,3))
        x = self.pred(x)
        return x
\end{lstlisting}

A high value of this metric implies that distinguishing the generated image from the authentic one is challenging for a simple network, indicating the high quality of generated images.

\section{More Experimental Results}
\subsection{Visualizations of Scene Text Editing}
We propose disentangled representation learning methods tailored for scene text tasks. Leveraging a disentangled training strategy, our model demonstrates competence in scene text editing tasks without the need for fine-tuning. we conduct a series of experiments to validate the effectiveness of our approach in Scene Text Editing (STE). Additionally, for more visualization of the generated quality, we present additional cases in \cref{fig:ste_more}. Specifically, in \cref{fig:ste_more} (a), we showcase the generation quality of our method, particularly in challenging scenes. In \cref{fig:ste_more} (b), we highlight our method's capability to follow various styles. For artistic texts or special style texts, our method can better retain the style of source images. In \cref{fig:ste_more} (c), we provide examples where both our method and MOSTEL~\cite{mostel} generate readable and clear images. However, our results exhibit greater realism, further supported by the ClassAcc metric test results.

\subsection{Inference Speed of Scene Text Recognition}
For Scene Text Recognition task, we fine-tune our model on Union-L \cite{union14m} dataset, and evaluate the model on both Common Benchmarks (CoB) \cite{IIIT,IC13,IC15,SVT,SVTP,CUTE} and Union14M-Benchmark (UnB) \cite{union14m}. These datasets are detailed in our main paper. Since the necessity for efficiency in deploying text recognition models, we assess the inference speed of our model in \cref{tab:speed}. SVTR \cite{svtr} and LPV \cite{LPV} stand out as two of the most efficient methods currently available. In comparison, our approach attains superior performance while preserving a minimal parameter count and ensuring high inference speed.

\begin{table}[]
\centering
\caption{Comparisons of the inference speed and parameter quantity in Scene Text Recognition. 'CoB AVG' means the average accuracy on common benchmarks \cite{IIIT,IC13,IC15,SVT,SVTP,CUTE}. 'UnB AVG' stands for the average accuracy on Union14M-Benchmark \cite{union14m}.}\label{tab:speed}
\resizebox{\columnwidth}{!}{%
\begin{tabular}{l|cccc}
\hline
Methods                    & CoB AVG       & \multicolumn{1}{l}{UnB AVG} & \# Paramter (M) & Speed (ms)    \\ \hline
SVTR-S~\cite{svtr}         & 91.1          & 68.4                        & \textbf{10.3}   & \textbf{4.81} \\
VisionLAN~\cite{visionlan} & 91.3          & 62.5                        & 33              & 21.73         \\
ABINet~\cite{abinet}       & 94.0          & 69.2                        & 37              & 46.86         \\
LPV-S~\cite{LPV}           & 95.2          & 78.0                        & 14              & 5.77          \\
DARLING (Ours)             & \textbf{95.6} & \textbf{80.2}               & 18.7            & 7.41          \\ \hline
\end{tabular}%
}
\end{table}

\subsection{Visualizations of Scene Text Removal}
We conduct fine-tuning of our model on the SCUT-EnsText \cite{enstext} dataset for the scene text removal task. Leveraging the advantages of our disentangled representation learning approach, our method demonstrates noteworthy performance improvements. Additional cases of our model are presented in \cref{fig:strm_more}. The results illustrate the capability of our model to achieve realistic erasure outcomes in both normal and challenging scenes.

\begin{figure*}[!h]
  \centering
   \includegraphics[width=1.0\linewidth]{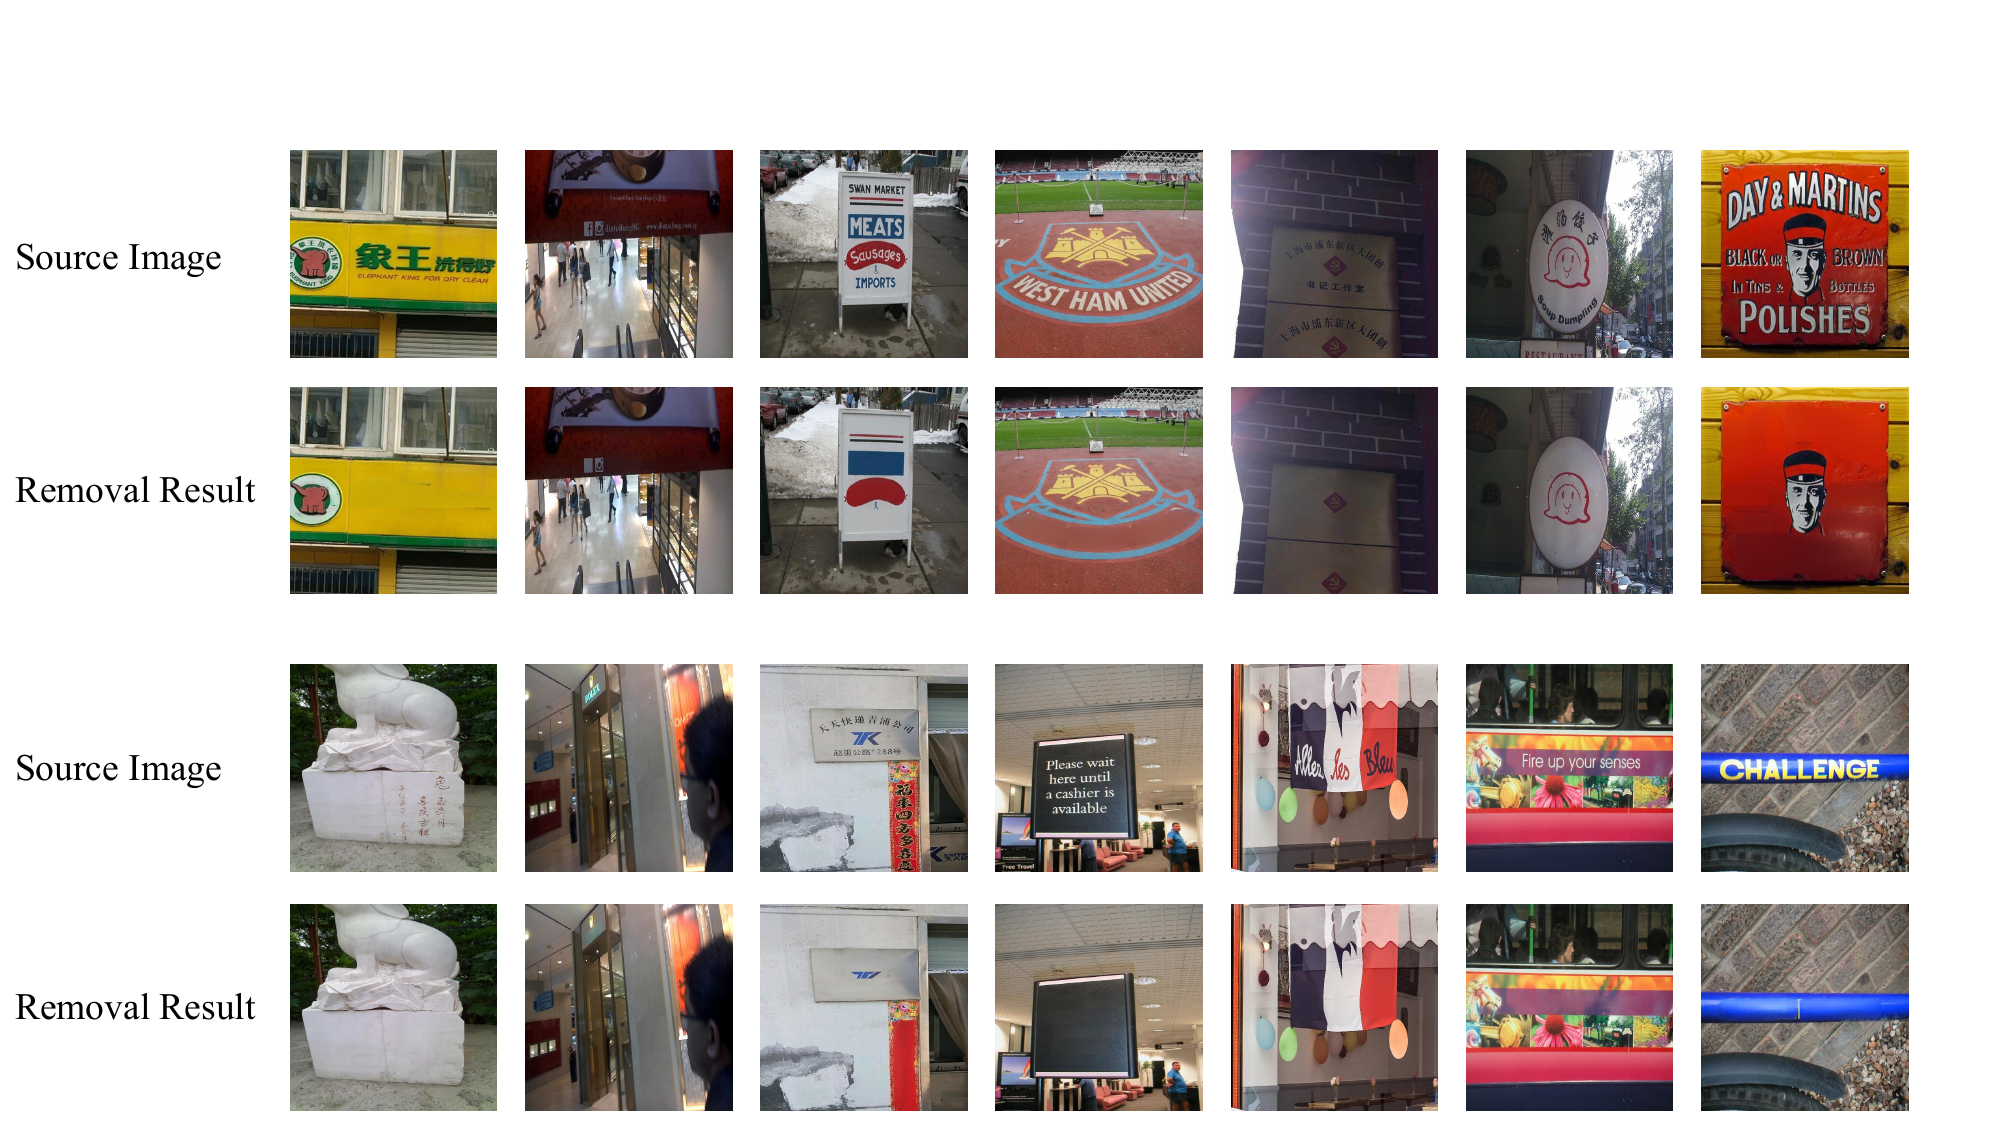}
   \caption{More visualizations of scene text removal results.}
   \label{fig:strm_more}
\end{figure*}
